# Supplementary material for: Frivolous Units: Wider Networks Are Not Really That Wide
Source: arXiv:1912.04783 source file (2021-05-31)
Supplement: Supplementary file 4 [file supp_data_mlp.tex]

\begin{figure*}[h!]
\centering
\begin{tabular}{cc}
	\includegraphics[width=.4\linewidth]{figures/acc_synth_data_test.pdf}&
	\includegraphics[width=.4\linewidth]{figures/auc_synthetic_data_test.pdf}\\
	(a) & (b)\\
	\includegraphics[width=.4\linewidth]{figures/comp_synthetic_data_test.pdf} &
	\includegraphics[width=.4\linewidth]{figures/sim_synth_data_test.pdf} \\
	(c) & (d)\\
\end{tabular}
\caption{\textbf{Varying training set size only affects compressibility amount in MLPs (Uncorrelated 10,000 dimensional synthetic data).} Trends in (a) accuracy, (b) robustness, (c) compressibility, and (d) similarity with various numbers of training examples across size factors for MLPs trained on 10,000 dimensional synthetic uncorrelated data.}
\label{fig:data_mlp}
\end{figure*}
