# Supplementary material for: Frivolous Units: Wider Networks Are Not Really That Wide
Source: arXiv:1912.04783 source file (2021-05-31)
Supplement: Supplementary file 11 [file supp_regularizers.tex]

\begin{figure*}[h!]
\centering
\begin{tabular}{ccc}
	\includegraphics[width=.3\linewidth]{figures/acc_cifar_regularizers_test.pdf}&
	\includegraphics[width=.3\linewidth]{figures/auc_cifar_regularizers_test.pdf}&
	\includegraphics[width=.3\linewidth]{figures/sim_cifar_regularizers_test.pdf} \\
	(a) & (b) & (c)\\
\end{tabular}
\caption{\textbf{Explicit regularization affects amounts but not trends for unit removability and similarity in AlexNets (CIFAR-10).} Trends in (a) accuracy, (b) removability, and (c) similarity with various explicit regularizers across size factors for AlexNets. We test data augmentation, dropout, weight decay, and all three together against the unregularized control. Each regularizer positively affects generalization performance, though weight decay only has a slightly positive effect. None serve to change the general trends in units removability and similarity, but they shift the curves up or down. Dropout and weight decay have a large and small positive effect on removability and similarity respectively. We attribute this to dropout forcing networks to develop redundant units to cope with ablations and weight decay pushing the weights of the network toward a smaller subspace.}
\label{fig:regs}
\end{figure*}
